# Supplementary material for: MaskingDepth: Masked Consistency Regularization for Semi-supervised Monocular Depth Estimation
Source: arXiv:2212.10806 source file (2023-03-23)
Supplement: Supplementary file 1 [file concat_ablation.tex]

\begin{table*}[t!]
\begin{minipage}{.5\linewidth}
    \centering
    \begin{tabular}{l|ccc}
            \toprule
            $K$ & AbsRel $\downarrow$ & RMSE $\downarrow$ &\textbf{$\delta$}$\uparrow$ \\
            \midrule
            $K=4$  &0.131 & 4.456 &0.850\\
            $K=16$ &0.128 & 4.298 &\textbf{0.855}\\
            $K=64$ &\textbf{0.124} & \textbf{4.263} &\textbf{0.855}\\
            $K=128$ &0.132 & 4.382 &0.849\\
            \bottomrule
    \end{tabular}%
    \caption{\textbf{Influence of the number of $K$.}}
    \label{tab:numberK}
\end{minipage}%
\begin{minipage}{.5\linewidth}
    \centering
    \begin{tabular}{c|c|c|c}
            \toprule
            Method & Blocks &  AbsRel $\downarrow$ & \textbf{$\delta$}$\uparrow$ \\
            \midrule
            w/o head       &- &0.317 &0.423\\
            Transformer    &1 &0.125 &\textbf{0.856}\\
            Transformer    &2 &0.129 &0.848\\
            MLP            &2 &\textbf{0.124} &0.855\\
            \bottomrule
    \end{tabular}
    \caption{\textbf{Comparison of using different predictor head.}}
    \label{tab:predictor}
\end{minipage}
\end{table*}
